# Supplementary material for: Adaptive Taxonomy Learning and Historical Patterns Modelling for Patent Classification
Source: arXiv:2308.05385 source file (2024-06-19)
Supplement: Supplementary file 1 [file Appendix.tex]

\appendix
\label{section-appendix}
In the appendix, details of the experiments are introduced.
